# Supplementary material for: SE-SLAM: Semi-Dense Structured Edge-Based Monocular SLAM
Source: arXiv:1909.03917 source file (2019-09-09)
Supplement: Supplementary file 1 [file appendix.tex]

%\subsection{SE3 Jacobian Expressions}

\subsection{Sequence usage details}

Table \ref{tbl:crop} shows starting frame (SF), stripped frames at the end (EF) and total number of frames (TF) for each of the sequences used.

\begin{table}[ht!]
	\centering
	%\small
	%\renewcommand{\arraystretch}{1.1}
	%\renewcommand{\tabcolsep}{3pt}
	\begin{tabular}{@{}lccc|lccc@{}}
		\hline\noalign{\smallskip}
		Seq& SF& EF& TF & Seq & SF& EF& TF \\
		\noalign{\smallskip}\hline\noalign{\smallskip}
		MH01&890&60&3682 &Room 1&80&0&2891\\
		MH02&750&60&3040 &Room 2&80&0&2891 \\
		MH03&350&60&2700 & Room 3&80&0&2891 \\
		MH04&400&60&2032 &Room 4&80&0&2882 \\
		MH05&410&60&2273 &Room 5&100&0&2821\\
		V101&110&70&2912 &Room 6&80&0&2828 \\
		V201&110&120&2280 &ICL-0&0&0&1508 \\
		V102&100&50&1710 &ICL-1 &0&0&966 \\
		V202&80&70&2348 & ICL-2&0&0& 881\\ 
		V203&-&-&2336 &ICL-3 &0&0& 1241\\
		V103&-&-&2149&&&&\\
		\noalign{\smallskip}
	\end{tabular}
	\caption{Sequence usage details} 
	\label{tbl:crop}
\end{table}
